# Supplementary material for: Towards Human-Interpretable Prototypes for Visual Assessment of Image Classification Models
Source: arXiv:2211.12173 source file (2022-11-22)

Prototype

Nearest training patches

Nearest test patches

Class 0

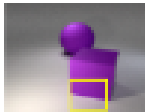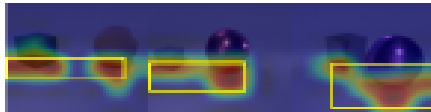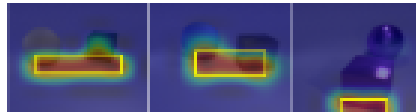

Class 1

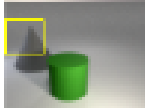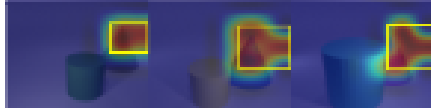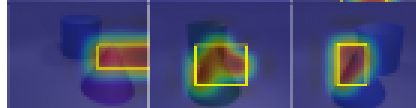

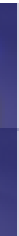

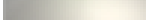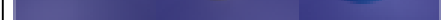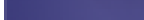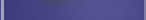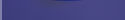

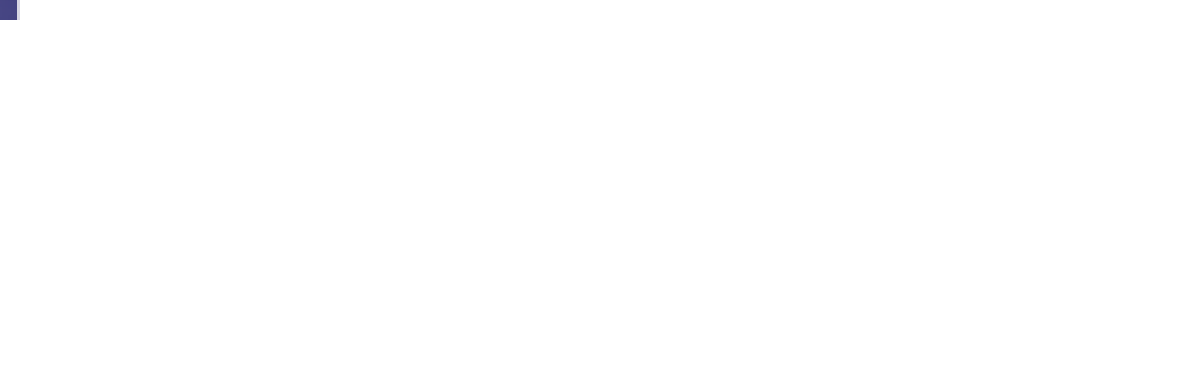

Supplement: Supplementary file 1 [file 3d_shapes_nearest_v2.pdf]
